# Supplementary material for: CRAG-MM-Diagnostics: Enabling Stage-Wise Analysis of Knowledge-Intensive VQA
Source: arXiv:2607.21155 source file (2026-07-23)
Supplement: Supplementary file 1 [file appendix_data_example.tex]

\definecolor{lightblue}{rgb}{233, 237, 201}

\definecolor{lightgray}{RGB}{237, 237, 233} % Define light gray color

\newpage
\begin{table}[ht!]
\centering
\caption{.}
\small
\resizebox{1.0\linewidth}{!}{
\begin{tabular}{m{1.5cm}m{3.5cm}m{3.5cm}m{2.1cm}>{\columncolor{lightgray}}m{3.5cm}>{\columncolor{lightgray}}m{2.1cm}}
        \toprule
        \multicolumn{2}{c}{Image} & \includegraphics[width=15mm,height=15mm]{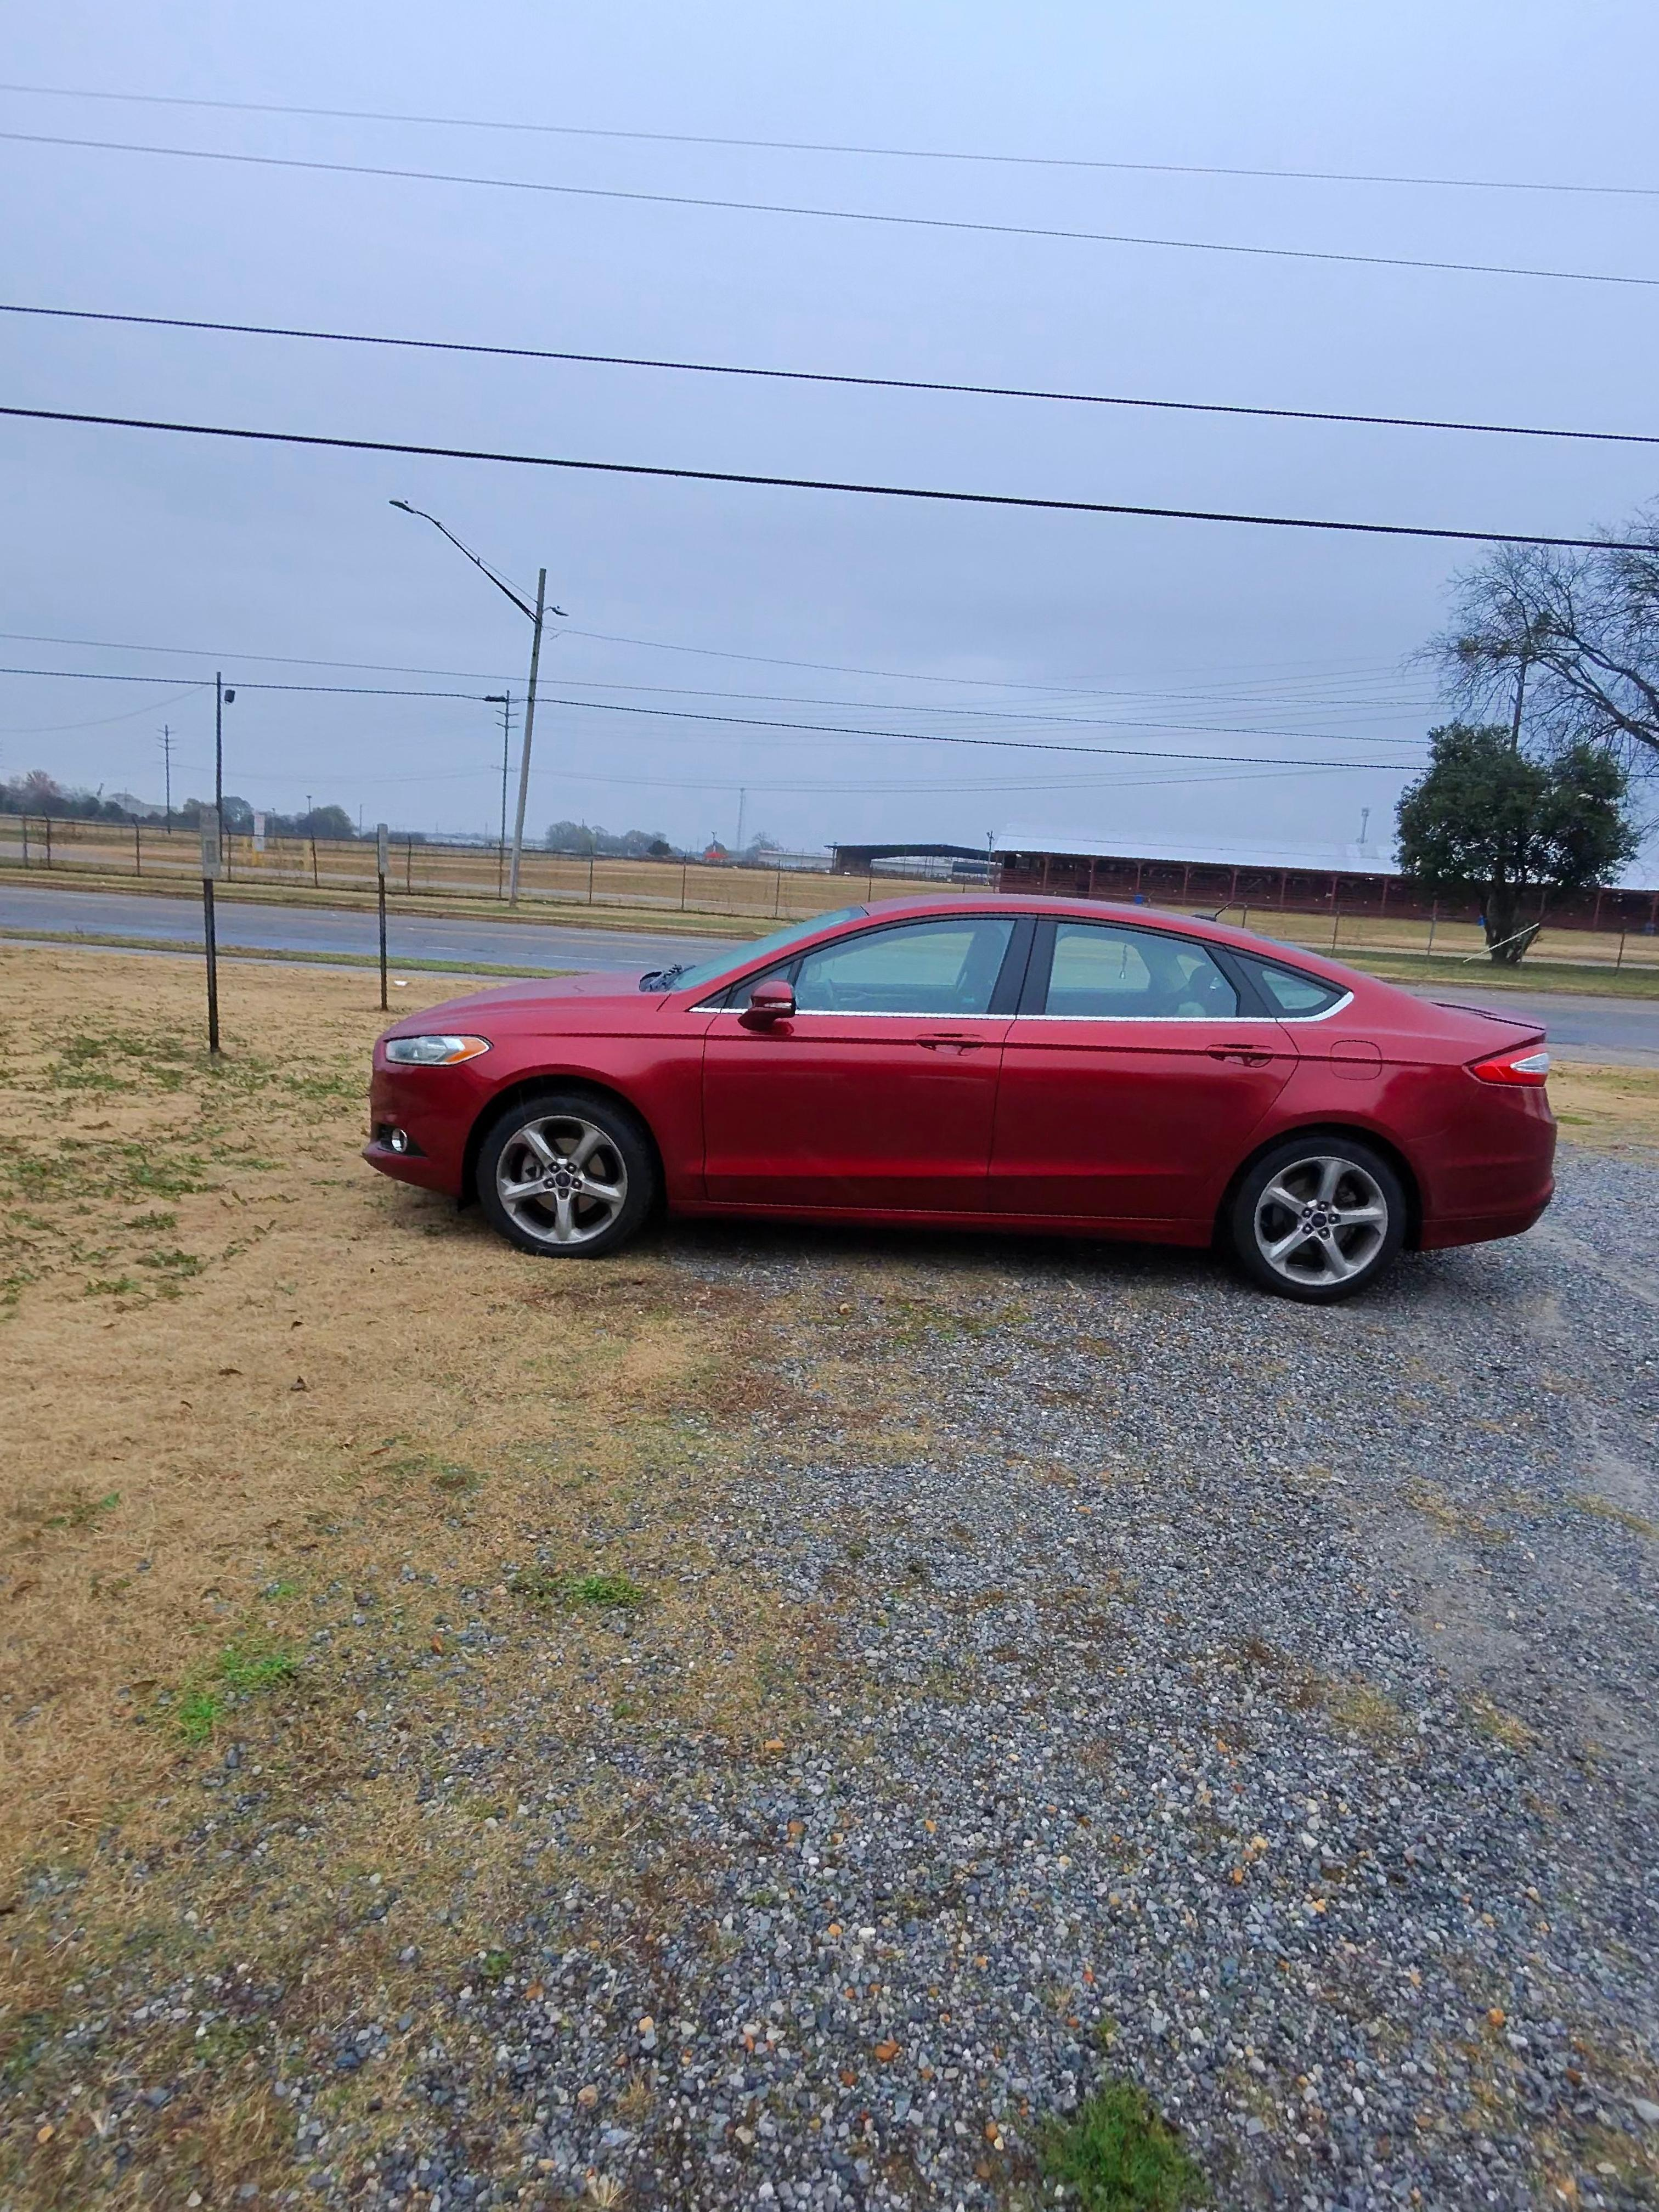}  \\
        \multicolumn{2}{c}{Question} & which came out first, this model or the ford focus?\\
        \multicolumn{2}{c}{Answer}& the ford focus, introduced in 1998, came out before the ford fusion, introduced in 2006.\\
        \midrule
        \multirow{4}{*}{Metadata}
         & Referring Expression & salient \\ 
         & Same Category Object Cnt & 1\\ 
         & Size of Target Object & 0.1411\\ 
         & Target ROI Box & [643,1610,2854,2388], \\ 
         & Target Object Name  & Ford Fusion (Americas)\\ 
         & Target Object Wiki URL & https://en.wikipedia.org/wiki/Ford_Fusion_(Americas) \\ 
         & Textual Only Question & Which came out first, the ford fusion or the ford focus? \\ 
         & Popularity & 296969 \\ 
         & Disambiguated Query & - \\
        \bottomrule
\end{tabular}
}
\label{tab:example}
\end{table}
